# Supplementary material for: Supporting Unified Shader Specialization by Co-opting C++ Features
Source: arXiv:2109.14682 ancillary file (2022-07-16)
Supplement: Supplementary file 1 [file UnifiedShaderProgramming-SupplementaryMaterial.pdf]

# Additional Background on Modern Shader Programming

KERRY A. SEITZ, JR., University of California, Davis, USA
THERESA FOLEY, NVIDIA, USA
SERBAN D. PORUMBESCU, University of California, Davis, USA
JOHN D. OWENS, University of California, Davis, USA

**Full Paper Citation:**
Kerry A. Seitz, Jr., Theresa Foley, Serban D. Porumbescu, and John D. Owens. 2022. Supporting Unified Shader Specialization by Co-opting C++ Features. *Proc. ACM Comput. Graph. Interact. Tech.* 5, 3, Article 25 (July 2022), 17 pages. https://doi.org/10.1145/3543866

## A INTRODUCTION

In this Supplementary Material, we define the services that a unified system needs to provide though the lens of modern real-time graphics programming. Often, graphics programmers use the term “shader” to refer to the code they write. The meaning of this term differs based on context, so we begin by defining how we use it and other related terminology in this work.

We define a *shader* as consisting of both *GPU shader code* that performs highly parallel rendering calculations and *host shader code* that provides an interface between GPU shader code and the rest of the application.[1] Since GPUs are coprocessors, invocation of GPU code must be initiated from host code running on a CPU. A *shader program* is an invocable unit of GPU code consisting of parameters, functions, and one or more entry points (further described in Section B). A shader program often provides compile-time configuration options called *specialization parameters*, and compiling the shader program with different values for those options generates multiple *shader variants* of the original code. A shader program’s corresponding host shader code is responsible for selecting which shader variant to invoke based on dynamic information available at application runtime, as well as coordinating data transfer between host memory and GPU memory to provide a shader program with its runtime parameters. A unified environment for real-time graphics programming needs to support both the host- and GPU-related aspects of shader programming.

In the next two sections, we discuss these two halves of shader code in more detail. We describe GPU shader code using HLSL and its programming model, but other shading languages like GLSL and Metal Shading Language are similar. We describe host shader code in the context of Unreal Engine 4 (UE4). While the graphics APIs provide underlying functionality necessary to interface between host and GPU code, most major game engines implement systems layered on top of these

[1]Many graphics programmers think of a “shader” as just the GPU code, but we believe it is useful to include the corresponding host code in the definition as well.

Authors’ addresses: Kerry A. Seitz, Jr., University of California, Davis, Department of Computer Science, One Shields Avenue, Davis, CA, 95616, USA, kaseitz@ucdavis.edu; Theresa Foley, NVIDIA, 2788 San Tomas Expressway, Santa Clara, CA, 95051, USA, tfoley@nvidia.com; Serban D. Porumbescu, University of California, Davis, Department of Electrical and Computer Engineering, One Shields Avenue, Davis, CA, 95616, USA, sdporumbescu@ucdavis.edu; John D. Owens, University of California, Davis, Department of Electrical and Computer Engineering, One Shields Avenue, Davis, CA, 95616, USA, jowens@ece.ucdavis.edu.

This work is licensed under a Creative Commons Attribution 4.0 International License.
© 2022 Copyright held by the owner/author(s).
2577-6193/2022/7-ART
https://doi.org/10.1145/3543866

```
#define LOW 0
#define MEDIUM 1
#define HIGH 2

Texture2D ColorTexture;
SamplerState ColorSampler;
RWTexture2D<float4> Output;


#if QUALITY == LOW
  float4 doFiltering(float2 pos) { /* Low Quality Method */ }
#elif QUALITY == MEDIUM
  float4 doFiltering(float2 pos) { /* Medium Quality Method */ }
#elif QUALITY == HIGH
  int ExtraParameter;
  float4 doFiltering(float2 pos) { /* High Quality Method */ }
#endif


[numthreads(8, 8, 1)]
void MainCS(uint2 DispatchThreadID : SV_DispatchThreadID) {
  float2 pixelPos = /* ... */;
  float4 outColor = ColorTexture.Sample(ColorSampler, pixelPos);

  for (int i = 0; i < ITERATION_COUNT; ++i) {
    outColor *= doFiltering(pixelPos);
  }

  Output[DispatchThreadID] = outColor;
}
```

Listing S-1. An example GPU shader program written in HLSL.

```
enum class QualityEnumType : int {
  Low,
  Medium,
  High
};

class FilterShaderCS : public FGlobalShader {
public:
  DECLARE_SHADER_TYPE(FilterShaderCS, Global);

  BEGIN_SHADER_PARAMETER_STRUCT(FParameters, )
    SHADER_PARAMETER_RDG_TEXTURE(Texture2D, ColorTexture)
    SHADER_PARAMETER_SAMPLER(SamplerState, ColorSampler)
    SHADER_PARAMETER_RDG_TEXTURE_UAV(RWTexture2D<float4>, Output)
    SHADER_PARAMETER(int, ExtraParameter)
  END_SHADER_PARAMETER_STRUCT()

  class QualityDimension :
    SHADER_PERMUTATION_ENUM_CLASS("QUALITY", QualityEnumType);

  class IterationCountDimension :
    SHADER_PERMUTATION_SPARSE_INT("ITERATION_COUNT", 2, 4, 8, 16);

  using FPermutationDomain = TShaderPermutationDomain<
    QualityDimension, IterationCountDimension>;
};

IMPLEMENT_GLOBAL_SHADER(FilterShaderCS,
  "/path/to/HLSL/file.usf", "MainCS", SF_Compute);
```

Listing S-2. Host shader code corresponding to the GPU shader program in Listing S-1. This code is written in C++ and uses features provided by UE4.

APIs to provide additional features aimed at making this task easier for their users. UE4's shader programming system puts significant emphasis on imposing structure on host shader code, which allows users to benefit from additional type checking and other static tools (e.g., the shader variant mechanism discussed in Section C). We choose to focus on UE4 for this discussion because this structure helps to clearly illustrate the host-related aspects of shader programming and, in many ways, represents the limits of what these systems can accomplish in a non-unified environment. Nevertheless, the tasks that UE4 host shader code must accomplish, as well as the issues it faces, are also applicable to other game engines and to the underlying graphics APIs.

## B GPU SHADER CODE

Listing S-1 shows an example of a typical shader program written in HLSL. Common practice is to modularize each GPU shader program as its own HLSL source file.[2] When invoked from host code, multiple *instances* of this program are executed in parallel, with each instance operating mostly independently.[3]

The shader program in Listing S-1 has an *entry point* function (`MainCS()` on line 21), which is where GPU code execution begins for each instance. Because this particular shader program is a compute shader, the entry point is annotated with information about how many threads to invoke per thread group (line 20).[4] This example also includes other GPU functions (e.g., the `doFiltering()` functions) that can be called from GPU code. In HLSL, an entry point may declare *varying parameters*, whose values can differ for each instance within an invocation. For example, each instance in a given invocation has a unique ID, and the `DispatchThreadID` varying parameter (line 21) provides an instance with its ID value. The value for this parameter is provided implicitly by the HLSL programming model; the code attaches the user-defined function parameter to the system-defined value using the HLSL "semantic" named `SV_DispatchThreadID`.

This shader program also has several *uniform parameters* (lines 5–7). Unlike varying parameters, the value of a uniform parameter is the same for all instances in a given invocation. For example, `ColorTexture` is a uniform parameter that represents a 2D image containing color information, and all instances within an invocation access the same 2D image when using this parameter.

The example in Listing S-1 also uses two *specialization parameters*: `QUALITY` and `ITERATION_COUNT`. Specialization parameters express the different compile-time options that are used to generate multiple shader variants of this shader program. Notice that these parameters are not declared explicitly in the GPU code, but their values are implicitly required for the shader program to compile properly. When compiling this program, the value for each parameter is passed in as a macro (i.e., a `#define`) for the C-style preprocessor that HLSL supports. As a result, the value for each specialization parameter is constant at compile-time in GPU code, which allows the compiler to better optimize the code (e.g., by unrolling the loop on line 25). Specialization parameters can also be used to define additional GPU functions and uniform parameters (e.g., the `ExtraParameter` uniform on line 15 is only defined when `QUALITY == HIGH`). Note that the possible values for `QUALITY` are also defined using the preprocessor (lines 1–3).

## C HOST SHADER CODE (IN UNREAL ENGINE 4)

Listing S-2 shows the UE4 host shader code corresponding to the example shader program in Listing S-1. In UE4, each shader program is accompanied by a C++ class (line 7) that provides the

[2]However, other files can be `#include`d to allow for reuse of HLSL code.
[3]The HLSL programming model provides some inter-instance synchronization and communication capabilities, but we will not discuss them here.
[4]For information about the HLSL compute shader programming model, as well as other types of shaders, we refer interested readers to the HLSL documentation: https://msdn.microsoft.com/en-us/library/windows/desktop/dn933277(v=vs.85).aspx.

host-side interface to the GPU code. The host code class is associated with a GPU shader program using a UE4 macro to indicate the filename of the HLSL code and name of the entry point function (lines 28–29).

The host code class includes declarations of the shader's uniform parameters using UE4's SHADER_PARAMETER macros (lines 11–16). These macros define a struct, which implements a strongly typed interface for passing parameter from host code to GPU code:

```
FilterShaderCS::FParameters* Parameters =
  /* allocate parameter struct */;

Parameters->ColorTexture = colorTexture;
Parameters->ColorSampler = colorSampler;
Parameters->Output = outputTexture;
```

Unlike in GPU shader code, host shader code in UE4 includes explicit declarations for specialization parameters (lines 18–22). Using the SHADER_PERMUTATION macros, programmers provide the system with a static set of options for each parameter (e.g., all values of an enum type or individual integer values). Then, these parameter declarations are used to create an FPermutationDomain for this shader (lines 24–25). This construct serves two purposes. First, at shader program compile time, it enables the UE4 system to statically generate all shader variants of the GPU shader program by using the statically specified set of options for each specialization parameter. Second, at game runtime, it enables host shader code to easily select which variant to invoke, based on runtime information:

```
FilterShaderCS::FPermutationDomain PermutationVector;
PermutationVector.Set<FilterShaderCS::QualityDimension>(quality);
PermutationVector.Set<FilterShaderCS::IterationCountDimension>(iterCount);
```

## D ISSUES IN A NON-UNIFIED ENVIRONMENT

At this point, we can identify several issues that arise as a result of a non-unified shader programming environment. These issues apply to both UE4 and other game engines, as well as to applications using the graphics APIs directly.

As shown in the example above, GPU and host code must both declare the uniform parameters that the shader needs (e.g., Listing S-1 lines 5–7 and Listing S-2 lines 11–16, respectively). Programmers must ensure that they use the same types and variable names in both declarations, and they must also keep these duplicate declarations consistent as the code changes. Similarly, host and GPU code cannot share types and functions in non-unified environments, leading to additional code duplication (e.g., the enum values in Listing S-2 lines 1–5 are redeclared in Listing S-1 lines 1–3). Failing to properly maintain consistency between host and GPU code can lead to runtime errors and bugs that are potentially difficult to track down and fix.

Additionally, note that in GPU code, specialization parameters are not explicitly defined. Instead, GPU code references these parameters and expects that they will be available at compile time. As a result, there is little verification—at either compile-time or runtime—that these parameters are referenced correctly (e.g., a typo in GPU code may result in a difficult-to-debug logic error). A programmer could easily #include GPU code that uses an implicit specialization parameter but

omit the corresponding declaration in the host code class, leaving future readers to wonder whether the omission is a mistake or if the default value is always correct for that particular shader.[5]

In contrast, in a unified system where host and GPU code share parameters, types, and functions, these kinds of issues do not exist. Unified systems can therefore reduce programmer burden and increase code robustness. However, the best way to support specialization in a unified shader programming environment is unclear. The difficulty arises from the need to compile-time specialize GPU shader code but then select which specializations to invoke based on information only available at runtime. Section 2 of the main paper discusses why the typical compile-time metaprogramming methods familiar to graphics programmers today (preprocessor-based methods and template metaprogramming) are insufficient for implementing specialization in a unified environment. Then, Section 3 describes our solution for supporting unified shader specialization: co-opting C++ attributes and virtual functions and implementing them with alternate semantics.

[5]We found ourselves in this exact scenario when looking through the UE4 codebase. A later commit added the parameter to the host code, confirming that the omission was a mistake: https://github.com/EpicGames/UnrealEngine/commit/2a2cebffe6a5a7164dbe2401ba2d5dd1901b649e
(Note: access to this page requires permission to access the UE4 source code on GitHub)
